# Supplementary material for: FOBE and HOBE: First- and High-Order Bipartite Embeddings
Source: arXiv:1905.10953 source file (2020-07-23)
Supplement: Supplementary file 1 [file appendix.tex]

% This section is supplied for reproducibility information

\begin{algorithm}[t]
\begin{algorithmic}[1]
\REQUIRE Hypergraph $H$, Samples per Object $s$, \\
         Sampled Neighbors $\gamma$, Algebraic Relaxation $a$\\
         Maximum Algebraic Distance $m$ \\
\ENSURE Lists $S_I$ and $S_O$ representing input and output samples
\FORALL{$n_i \in H_N$, $n_j \in N^s \sim \Gamma(\Gamma(n_i))$}
\label{alg:algebraic_hypergraph2vec_sampling:node_node:loop}
    \STATE{Append $\left(n_i, n_j, 0, 0, \vv{0}^\gamma, \vv{0}^\gamma\right)$ to $S_I$}\\
    \STATE{Append $\left(\textsc{AlgSim}(n_i, n_j, a, m), 0, 0\right)$ to $S_O$}
\ENDFOR
\FORALL{$e_i \in H_E$, $e_j \in E^s \sim \Gamma(\Gamma(e_i))$}
\label{alg:algebraic_hypergraph2vec_sampling:edge_edge:loop}
    \STATE{Append $\left(0, 0, e_i, e_j, \vv{0}^\gamma, \vv{0}^\gamma\right)$ to $S_I$}
    \STATE{Append $\left(0, \textsc{AlgSim}(e_i, e_j, a, m), 0\right)$ to $S_O$}
\ENDFOR
\FORALL{$n \in H_N$, $e \in E^s \sim \Gamma(\Gamma(\Gamma(n)))$ \\
    \AND $e\in H_E$, $n \in N^s \sim \Gamma(\Gamma(\Gamma(e)))$}
\label{alg:algebraic_hypergraph2vec_sampling:node_edge:loop}
    \STATE{Append $\left(n, 0, e, 0, 
                         N^{\gamma} \sim \Gamma(e), 
                         E^{\gamma} \sim \Gamma(n) \right)$
           to $S_I$}
    \STATE{$v \leftarrow \underset{e' \in \Gamma(n)}{\max}{\textsc{AlgSim}(e', e, a, m)}$}
    \label{alg:algebraic_hypergraph2vec_sampling:node_edge_similarity}
    \STATE{Append $\left(0, 0, v\right)$ to $S_O$}
\ENDFOR

\end{algorithmic}
\caption{Algebraic Hypergraph2Vec Sampling}
\label{alg:algebraic_hypergraph2vec_sampling}
\end{algorithm}

\begin{algorithm}[t]
\begin{algorithmic}[1]
\REQUIRE Same typed indices $x$ and $y$, Algebraic Relaxation $a$, \\
        Maximal Algebraic Distance $m$ 
\ENSURE Observed $x,y$ similarity $v$
\STATE{$v \leftarrow 0$}
\FORALL{$z \in \Gamma(x) \cap \Gamma(y)$}
    \STATE{$w_x \leftarrow \left(m - ||a(x) - a(z)||_2\right) / m)$}\\
    \label{alg:algebraic_same_type_sample:weight_x}
    \STATE{$w_y \leftarrow \left(m - ||a(y) - a(z)||_2\right) / m)$}\\
    \label{alg:algebraic_same_type_sample:weight_y}
    \STATE{$v \leftarrow \max(\min(w_x, w_y))$}
    \label{alg:algebraic_same_type_sample:max_min}
\ENDFOR
\RETURN $v$
\end{algorithmic}
\caption{Same-Type Algebraic Similarity (\textsc{AlgSim})}
\label{alg:algebraic_same_type_sample}
\end{algorithm}

% Boolean Sampling Algorithm
\begin{algorithm}[t]
\begin{algorithmic}[1]
\REQUIRE Graph $G=(A \cup B,E)$, \\
         Samples per Node $s$, \\
         Number of Sampled Neighbors $\gamma$\\
\ENSURE Lists $S_I$ and $S_O$ representing input and output samples
\FORALL{$n_i \in N$, $n_j \in N^s \sim \Gamma(\Gamma(n_i))$}
\label{alg:boolean_hypergraph2vec_sampling:node_node}
        \STATE{Append $\left(n_i, n_j, 0, 0, \vv{0}^\gamma, \vv{0}^\gamma\right)$ to $S_I$}
        \STATE{Append $\left(1, 0, 0\right)$ to $S_O$}
\ENDFOR
\FORALL{$e_i \in E$, $e_j \in E^s \sim \Gamma(\Gamma(e_i))$}
\label{alg:boolean_hypergraph2vec_sampling:edge_edge}
        \STATE{Append $\left(0, 0, e_i, e_j, \vv{0}^\gamma, \vv{0}^\gamma\right)$ to $S_I$}
        \STATE{Append $\left(0, 1, 0\right)$ to $S_O$}
\ENDFOR
\FORALL{$n \in N$, $e \in E^s \sim \Gamma(n)$
   \AND $e\in E$, $n \in N^s \sim \Gamma(e)$}
\label{alg:boolean_hypergraph2vec_sampling:node_edge}
        \STATE{Append $\left(n, 0, e, 0, N^{\gamma} \sim \Gamma(e), E^{\gamma} \sim \Gamma(n) \right)$ to $S_I$}
        \STATE{Append $\left(0, 0, 1\right)$ to $S_O$}
\ENDFOR

\end{algorithmic}
\caption{Sampling for FOBE}
\label{alg:boolean_hypergraph2vec_sampling}
\end{algorithm}
